# Supplementary material for: Qubit Mapping Based on Subgraph Isomorphism and Filtered Depth-Limited Search
Source: arXiv:2004.07138 source file (2021-09-22)
Supplement: Supplementary file 1 [file appendix.tex]

% Please add the following required packages to your document preamble:
% \usepackage{longtable}
% Note: It may be necessary to compile the document several times to get a multi-page table to line up properly

{
\small
\begin{longtable}{ccc|cccc|cc}
\hline
\begin{tabular}[c]{@{}c@{}}Circuit\\   name\end{tabular} & \begin{tabular}[c]{@{}c@{}}qubit\\ no.\end{tabular} & \begin{tabular}[c]{@{}c@{}}input \\ CNOT\end{tabular} & \begin{tabular}[c]{@{}c@{}}topgr.\\ added\end{tabular} & \begin{tabular}[c]{@{}c@{}}wgtgr.\\ added\end{tabular} & \begin{tabular}[c]{@{}c@{}}empty\\ added\end{tabular} & \begin{tabular}[c]{@{}c@{}}naive\\ added\end{tabular} & \begin{tabular}[c]{@{}c@{}}\textsc{sahs}\\ added\end{tabular} & \multicolumn{1}{c}{\begin{tabular}[c]{@{}c@{}}Cambridge\\ added\end{tabular}} \\ \hline
\endhead
ex1\_226 & 6 & 5 & 0 & 0 & 3 & 18 & 0 & 0 \\
graycode6\_47 & 6 & 5 & 0 & 0 & 0 & 9 & 0 & 0 \\
xor5\_254 & 6 & 5 & 0 & 0 & 3 & 18 & 0 & 0 \\
4gt11\_84 & 4 & 9 & 0 & 0 & 9 & 12 & 0 & 0 \\
ex-1\_166 & 3 & 9 & 0 & 0 & 6 & 6 & 0 & 0 \\
4mod5-v0\_20 & 5 & 10 & 0 & 0 & 9 & 9 & 0 & 9 \\
4mod5-v1\_22 & 5 & 11 & 0 & 0 & 9 & 12 & 0 & 9 \\
ham3\_102 & 3 & 11 & 0 & 0 & 9 & 6 & 0 & 0 \\
mod5d1\_63 & 5 & 13 & 0 & 0 & 3 & 12 & 0 & 0 \\
4gt11\_83 & 5 & 14 & 0 & 0 & 0 & 18 & 0 & 12 \\
4mod5-v0\_19 & 5 & 16 & 0 & 0 & 0 & 18 & 0 & 9 \\
4mod5-v1\_24 & 5 & 16 & 0 & 0 & 15 & 21 & 0 & 12 \\
mod5mils\_65 & 5 & 16 & 0 & 0 & 15 & 21 & 0 & 9 \\
rd32-v0\_66 & 4 & 16 & 0 & 0 & 18 & 18 & 0 & 0 \\
rd32-v1\_68 & 4 & 16 & 0 & 0 & 18 & 18 & 0 & 0 \\
3\_17\_13 & 3 & 17 & 0 & 0 & 9 & 9 & 0 & 0 \\
alu-v0\_27 & 5 & 17 & 9 & 6 & 12 & 18 & 6 & 3 \\
alu-v1\_29 & 5 & 17 & 9 & 6 & 12 & 24 & 6 & 3 \\
alu-v2\_33 & 5 & 17 & 9 & 6 & 12 & 18 & 6 & 9 \\
4gt11\_82 & 5 & 18 & 3 & 3 & 3 & 27 & 3 & 12 \\
alu-v1\_28 & 5 & 18 & 9 & 6 & 21 & 18 & 6 & 3 \\
alu-v3\_35 & 5 & 18 & 9 & 6 & 12 & 24 & 6 & 3 \\
alu-v4\_37 & 5 & 18 & 9 & 6 & 12 & 18 & 6 & 3 \\
decod24-v2\_43 & 4 & 22 & 0 & 0 & 18 & 15 & 0 & 0 \\
decod24-v0\_38 & 4 & 23 & 0 & 0 & 27 & 15 & 0 & 0 \\
miller\_11 & 3 & 23 & 0 & 0 & 6 & 9 & 0 & 0 \\
alu-v3\_34 & 5 & 24 & 9 & 6 & 27 & 27 & 6 & 3 \\
mod5d2\_64 & 5 & 25 & 18 & 9 & 18 & 36 & 12 & 12 \\
4gt13\_92 & 5 & 30 & 0 & 0 & 30 & 42 & 0 & 18 \\
4gt13-v1\_93 & 5 & 30 & 0 & 0 & 33 & 27 & 0 & 18 \\
4mod5-bdd\_287 & 7 & 31 & 6 & 18 & 9 & 36 & 6 & 15 \\
4mod5-v0\_18 & 5 & 31 & 9 & 12 & 30 & 36 & 9 & 9 \\
4mod5-v1\_23 & 5 & 32 & 9 & 21 & 30 & 36 & 9 & 12 \\
decod24-bdd\_294 & 6 & 32 & 15 & 27 & 24 & 24 & 15 & 21 \\
one-two-three-v2\_100 & 5 & 32 & 9 & 9 & 18 & 30 & 9 & 9 \\
one-two-three-v3\_101 & 5 & 32 & 15 & 18 & 24 & 36 & 6 & 15 \\
rd32\_270 & 5 & 36 & 18 & 24 & 39 & 30 & 12 & 18 \\
4gt5\_75 & 5 & 38 & 9 & 12 & 24 & 51 & 15 & 15 \\
alu-bdd\_288 & 7 & 38 & 24 & 15 & 39 & 36 & 24 & 45 \\
alu-v0\_26 & 5 & 38 & 12 & 9 & 30 & 36 & 9 & 21 \\
decod24-v1\_41 & 5 & 38 & 3 & 21 & 21 & 45 & 15 & 18 \\
4gt5\_76 & 5 & 46 & 21 & 36 & 48 & 48 & 15 & 27 \\
4gt13\_91 & 5 & 49 & 6 & 6 & 15 & 45 & 15 & 6 \\
alu-v4\_36 & 5 & 51 & 6 & 15 & 30 & 30 & 15 & 36 \\
4gt13\_90 & 5 & 53 & 9 & 9 & 18 & 48 & 27 & 9 \\
4gt5\_77 & 5 & 58 & 9 & 18 & 18 & 45 & 9 & 36 \\
one-two-three-v1\_99 & 5 & 59 & 24 & 33 & 42 & 48 & 12 & 39 \\
rd53\_138 & 8 & 60 & 30 & 42 & 30 & 42 & 27 & 39 \\
decod24-v3\_45 & 5 & 64 & 15 & 24 & 36 & 72 & 15 & 39 \\
one-two-three-v0\_98 & 5 & 65 & 18 & 27 & 48 & 63 & 24 & 27 \\
4gt10-v1\_81 & 5 & 66 & 15 & 18 & 36 & 60 & 27 & 33 \\
aj-e11\_165 & 5 & 69 & 33 & 36 & 42 & 33 & 18 & 24 \\
4mod7-v0\_94 & 5 & 72 & 12 & 27 & 33 & 51 & 12 & 39 \\
4mod7-v1\_96 & 5 & 72 & 21 & 21 & 48 & 45 & 18 & 42 \\
alu-v2\_32 & 5 & 72 & 15 & 45 & 69 & 45 & 15 & 39 \\
mod10\_176 & 5 & 78 & 15 & 24 & 63 & 66 & 24 & 36 \\
4gt4-v0\_80 & 6 & 79 & 15 & 39 & 48 & 69 & 24 & 78 \\
cnt3-5\_179 & 16 & 85 & 3 & 30 & 72 & 87 & 15 & 87 \\
4gt12-v0\_88 & 6 & 86 & 21 & 15 & 69 & 66 & 21 & 21 \\
ising\_model\_10 & 10 & 90 & 0 & 0 & 18 & 27 & 0 & 0 \\
qft\_10 & 10 & 90 & 45 & 33 & 57 & 96 & 36 & 57 \\
sys6-v0\_111 & 10 & 98 & 54 & 81 & 63 & 60 & 45 & 111 \\
4\_49\_16 & 5 & 99 & 18 & 30 & 42 & 48 & 36 & 69\\
\hline

sum	& & 2428    & 618	& 849	& 1602	& 2133 &	636	&	1239\\	
I-index	&  &  &   1.255 &	1.350 &	1.660 &	1.879 &	1.262 &	1.510 \\	
%I-index &  &  & 1.254530478	1.349670511	1.659802306	1.878500824	1.261943987		1.51029654	
\hline
\caption{Comparison on IBM Q Tokyo with small circuits}
\label{tab:extra-small}\\
\end{longtable}

\vspace*{-5mm}
% Please add the following required packages to your document preamble:
% \usepackage{longtable}
% Note: It may be necessary to compile the document several times to get a multi-page table to line up properly
\begin{longtable}{ccc|cccc|cc}
\hline
\begin{tabular}[c]{@{}c@{}}Circuit\\   name\end{tabular} & \begin{tabular}[c]{@{}c@{}}qubit\\ no.\end{tabular} & \begin{tabular}[c]{@{}c@{}}input \\ CNOT\end{tabular} & \begin{tabular}[c]{@{}c@{}}topgr.\\ added\end{tabular} & \begin{tabular}[c]{@{}c@{}}wgtgr.\\ added\end{tabular} & \begin{tabular}[c]{@{}c@{}}empty\\ added\end{tabular} & \begin{tabular}[c]{@{}c@{}}naive\\ added\end{tabular} & \begin{tabular}[c]{@{}c@{}}\textsc{sahs}\\ added\end{tabular} & \multicolumn{1}{c}{\begin{tabular}[c]{@{}c@{}}Cambridge\\ added\end{tabular}} \\ \hline
\endhead
4gt12-v1\_89 & 6 & 100 & 57 & 18 & 30 & 81 & 24 & 93 \\
0410184\_169 & 14 & 104 & 6 & 27 & 75 & 93 & 12 & 75 \\
4gt4-v0\_79 & 6 & 105 & 12 & 12 & 30 & 87 & 12 & 96 \\
hwb4\_49 & 5 & 107 & 36 & 42 & 54 & 63 & 33 & 45 \\
mod10\_171 & 5 & 108 & 39 & 27 & 27 & 60 & 24 & 60 \\
4gt4-v0\_78 & 6 & 109 & 15 & 15 & 33 & 93 & 15 & 99 \\
4gt12-v0\_87 & 6 & 112 & 6 & 6 & 24 & 69 & 6 & 123 \\
4gt4-v0\_72 & 6 & 113 & 45 & 39 & 51 & 93 & 42 & 90 \\
4gt12-v0\_86 & 6 & 116 & 9 & 9 & 27 & 75 & 9 & 123 \\
4gt4-v1\_74 & 6 & 119 & 39 & 27 & 75 & 93 & 78 & 114 \\
ising\_model\_13 & 13 & 120 & 0 & 0 & 36 & 45 & 0 & 0 \\
mini-alu\_167 & 5 & 126 & 30 & 33 & 69 & 87 & 33 & 75 \\
one-two-three-v0\_97 & 5 & 128 & 42 & 78 & 72 & 90 & 66 & 66 \\
rd53\_135 & 7 & 134 & 60 & 84 & 99 & 111 & 54 & 48 \\
decod24-enable\_126 & 6 & 149 & 66 & 63 & 72 & 84 & 87 & 81 \\
ham7\_104 & 7 & 149 & 48 & 42 & 75 & 51 & 81 & 102 \\
ising\_model\_16 & 16 & 150 & 0 & 0 & 48 & 48 & 0 & 0 \\
mod8-10\_178 & 6 & 152 & 69 & 33 & 69 & 87 & 21 & 162 \\
rd84\_142 & 15 & 154 & 84 & 126 & 87 & 108 & 102 & 198 \\
ex3\_229 & 6 & 175 & 24 & 81 & 87 & 102 & 18 & 174 \\
4gt4-v0\_73 & 6 & 179 & 99 & 42 & 117 & 120 & 42 & 177 \\
mod8-10\_177 & 6 & 196 & 123 & 78 & 72 & 87 & 39 & 135 \\
alu-v2\_31 & 5 & 198 & 78 & 90 & 60 & 99 & 54 & 63 \\
rd53\_131 & 7 & 200 & 63 & 78 & 93 & 81 & 90 & 87 \\
C17\_204 & 7 & 205 & 111 & 84 & 144 & 147 & 96 & 114 \\
alu-v2\_30 & 6 & 223 & 60 & 54 & 87 & 93 & 45 & 105 \\
mod5adder\_127 & 6 & 239 & 84 & 81 & 93 & 114 & 51 & 87 \\
qft\_16 & 16 & 240 & 189 & 135 & 204 & 231 & 135 & 195 \\
rd53\_133 & 7 & 256 & 60 & 174 & 138 & 150 & 105 & 159 \\
majority\_239 & 7 & 267 & 66 & 105 & 87 & 213 & 84 & 123 \\
ex2\_227 & 7 & 275 & 78 & 108 & 90 & 126 & 96 & 270 \\
cm82a\_208 & 8 & 283 & 117 & 105 & 102 & 225 & 84 & 222 \\
sf\_274 & 6 & 336 & 30 & 36 & 63 & 180 & 24 & 381 \\
sf\_276 & 6 & 336 & 36 & 36 & 102 & 159 & 24 & 384 \\
con1\_216 & 9 & 415 & 273 & 153 & 210 & 195 & 192 & 375 \\
rd53\_130 & 7 & 448 & 267 & 207 & 168 & 222 & 171 & 390 \\
f2\_232 & 8 & 525 & 336 & 126 & 192 & 312 & 213 & 225 \\
rd53\_251 & 8 & 564 & 201 & 195 & 225 & 240 & 204 & 309 \\
hwb5\_53 & 6 & 598 & 207 & 204 & 195 & 237 & 174 & 210 \\ \hline
sum &  & 8513 & 3165 & 2853 & 3582 & 4851 & 2640 & 5835 \\
I-index &  &  & 1.372 & 1.335 & 1.421 & 1.570 & 1.310 & 1.685
%I-index &  &  & 1.37178433 & 1.3351345 & 1.420768237 & 1.569834371 & 1.310113943 & 1.685422295
\\
\hline

\caption{Comparison on IBM Q Tokyo with  medium circuits}
\label{tab:extra-medium}
\end{longtable}

\vspace*{-5mm}
% Please add the following required packages to your document preamble:
% \usepackage{longtable}
% Note: It may be necessary to compile the document several times to get a multi-page table to line up properly
\begin{longtable}{ccc|cccc|cc}
\hline
\begin{tabular}[c]{@{}c@{}}Circuit\\   name\end{tabular} & \begin{tabular}[c]{@{}c@{}}qubit\\ no.\end{tabular} & \begin{tabular}[c]{@{}c@{}}input \\ CNOT\end{tabular} & \begin{tabular}[c]{@{}c@{}}topgr.\\ added\end{tabular} & \begin{tabular}[c]{@{}c@{}}wgtgr.\\ added\end{tabular} & \begin{tabular}[c]{@{}c@{}}empty\\ added\end{tabular} & \begin{tabular}[c]{@{}c@{}}naive\\ added\end{tabular} & \begin{tabular}[c]{@{}c@{}}\textsc{sahs}\\ added\end{tabular} & \multicolumn{1}{c}{\begin{tabular}[c]{@{}c@{}}Cambridge\\ added\end{tabular}} \\ \hline
\endhead
z4\_268 & 11 & 1343 & 525 & 468 & 609 & 600 & 546 & 1671 \\
radd\_250 & 13 & 1405 & 633 & 567 & 555 & 549 & 669 & 1647 \\
adr4\_197 & 13 & 1498 & 681 & 741 & 642 & 807 & 711 & 1146 \\
sym6\_145 & 7 & 1701 & 540 & 585 & 540 & 765 & 744 & 2139 \\
misex1\_241 & 15 & 2100 & 621 & 726 & 858 & 924 & 921 & 1263 \\
rd73\_252 & 10 & 2319 & 1062 & 852 & 1227 & 1074 & 1065 & 2115 \\
cycle10\_2\_110 & 12 & 2648 & 1125 & 1290 & 1320 & 1236 & 1038 & 2424 \\
hwb6\_56 & 7 & 2952 & 1077 & 1026 & 1098 & 1011 & 1104 & 1719 \\
square\_root\_7 & 15 & 3089 & 1263 & 1374 & 1242 & 1470 & 1353 & 1326 \\
sqn\_258 & 10 & 4459 & 1467 & 1716 & 1638 & 1986 & 1953 & 3192 \\
cm85a\_209 & 14 & 4986 & 2073 & 2091 & 2289 & 2397 & 2337 & 4173 \\
rd84\_253 & 12 & 5960 & 2952 & 2841 & 3174 & 3009 & 3198 & 5286 \\
root\_255 & 13 & 7493 & 2928 & 3099 & 3468 & 3399 & 3525 & 5601 \\
co14\_215 & 15 & 7840 & 3975 & 4563 & 4629 & 4437 & 4356 & 7752 \\
mlp4\_245 & 16 & 8232 & 4275 & 4146 & 4173 & 4104 & 4116 & 6462 \\
sym9\_148 & 10 & 9408 & 1947 & 2166 & 1992 & 2388 & 2172 & 6438 \\
urf2\_277 & 8 & 10066 & 6285 & 6267 & 6135 & 6045 & 5934 & 8205 \\
hwb7\_59 & 8 & 10681 & 3684 & 3846 & 3696 & 3588 & 4602 & 6378 \\
max46\_240 & 10 & 11844 & 4410 & 4308 & 4560 & 4530 & 5289 & 9681 \\
clip\_206 & 14 & 14772 & 6762 & 6834 & 6963 & 6405 & 6843 & 12624 \\
9symml\_195 & 11 & 15232 & 5481 & 6462 & 5373 & 5682 & 6036 & 11454 \\
sym9\_193 & 11 & 15232 & 5481 & 6462 & 5373 & 5682 & 6123 & 11454 \\
dist\_223 & 13 & 16624 & 7470 & 6582 & 7107 & 7254 & 6936 & 12834 \\
sao2\_257 & 14 & 16864 & 7596 & 6756 & 8361 & 6792 & 7827 & 11742 \\
urf5\_280 & 9 & 23764 & 11988 & 11679 & 12060 & 11802 & 13065 & 20436 \\
urf1\_278 & 9 & 26692 & 13872 & 13809 & 14190 & 14022 & 15678 & 24600 \\
sym10\_262 & 12 & 28084 & 11490 & 10623 & 11520 & 10635 & 11697 & 20115 \\
hwb8\_113 & 9 & 30372 & 11295 & 11382 & 11769 & 11394 & 14976 & 35376 \\ %59977=>14976
urf2\_152 & 8 & 35210 & 18342 & 18342 & 18018 & 18489 & 18780 & 25857 \\ \hline
sum &  & 322870 & 141300 & 141603 & 144579 & 142476 & 153594 & 265110 \\ %198595 => 198595 -(59977-14976) = 153594
I-index &  &  & 1.438 & 1.439 & 1.448 & 1.441 & 1.476 & 1.821 %1.615 => 1.476
%I-index &  &  & 1.437637439 & 1.438575897 & 1.447793229 & 1.441279772 & 1.615092762 & 1.821104469
\\
\hline
\caption{Comparison on IBM Q Tokyo with  large circuits }
\label{tab:extra-large}
\end{longtable}
}
