# Supplementary material for: Qubit Mapping Based on Subgraph Isomorphism and Filtered Depth-Limited Search
Source: arXiv:2004.07138 source file (2021-09-22)
Supplement: Supplementary file 2 [file appendixA.tex]

{
\small
%\begin{longtable}{ccc|ccc|ccc|ccc}

\begin{longtable}{ cc*{9}{c|}c }
    \hline
     \multicolumn{3}{c|}{circ. info}
                    & \multicolumn{3}{c|}{topgraph initial mapping}
                    & \multicolumn{3}{c|}{G with other mappings}
                    & \multicolumn{3}{c}{other algorithms}\\ 

\hline
name & \#q & \#CX & G & GQ01x & D & wgtgr. & empty & naive & \sabre &
camb. & 
\sahs \\ \hline
	ex1\_226 & 6 & 5 & 0 & 0 & 0 & 0 & 3 & 18 & 0 & 0 & 0 \\ \hline
	graycode6\_47 & 6 & 5 & 0 & 0 & 0 & 0 & 0 & 9 & 0 & 0 & 0 \\ \hline
	xor5\_254 & 6 & 5 & 0 & 0 & 0 & 0 & 3 & 18 & 0 & 0 & 0 \\ \hline
	ex-1\_166 & 3 & 9 & 0 & 0 & 0 & 0 & 6 & 6 & 0 & 0 & 0 \\ \hline
	4gt11\_84 & 4 & 9 & 0 & 0 & 0 & 0 & 9 & 9 & 0 & 0 & 0 \\ \hline
	4mod5-v0\_20 & 5 & 10 & 0 & 0 & 0 & 0 & 0 & 9 & 3 & 9 & 0 \\ \hline
	ham3\_102 & 3 & 11 & 0 & 0 & 0 & 0 & 9 & 6 & 0 & 9 & 0 \\ \hline
	4mod5-v1\_22 & 5 & 11 & 0 & 0 & 0 & 0 & 0 & 12 & 0 & 0 & 0 \\ \hline
	mod5d1\_63 & 5 & 13 & 0 & 0 & 0 & 0 & 0 & 12 & 0 & 0 & 0 \\ \hline
	4gt11\_83 & 5 & 14 & 0 & 0 & 0 & 0 & 0 & 18 & 0 & 12 & 0 \\ \hline
	rd32-v1\_68 & 4 & 16 & 0 & 0 & 0 & 0 & 18 & 18 & 0 & 9 & 0 \\ \hline
	rd32-v0\_66 & 4 & 16 & 0 & 0 & 0 & 0 & 18 & 18 & 9 & 12 & 0 \\ \hline
	4mod5-v1\_24 & 5 & 16 & 0 & 0 & 0 & 0 & 18 & 21 & 0 & 9 & 0 \\ \hline
	4mod5-v0\_19 & 5 & 16 & 0 & 0 & 0 & 0 & 0 & 18 & 0 & 0 & 0 \\ \hline
	mod5mils\_65 & 5 & 16 & 0 & 0 & 0 & 0 & 0 & 21 & 9 & 0 & 0 \\ \hline
	alu-v1\_29 & 5 & 17 & 9 & 9 & 9 & 6 & 6 & 24 & 0 & 0 & 0 \\ \hline
	alu-v2\_33 & 5 & 17 & 9 & 9 & 9 & 6 & 6 & 18 & 3 & 3 & 6 \\ \hline
	alu-v0\_27 & 5 & 17 & 9 & 9 & 9 & 6 & 6 & 18 & 3 & 3 & 6 \\ \hline
	3\_17\_13 & 3 & 17 & 0 & 0 & 0 & 0 & 9 & 9 & 9 & 9 & 6 \\ \hline
	alu-v1\_28 & 5 & 18 & 9 & 9 & 9 & 6 & 6 & 18 & 3 & 12 & 3 \\ \hline
	alu-v4\_37 & 5 & 18 & 9 & 9 & 9 & 6 & 6 & 18 & 3 & 3 & 6 \\ \hline
	alu-v3\_35 & 5 & 18 & 9 & 9 & 9 & 6 & 6 & 24 & 3 & 3 & 6 \\ \hline
	4gt11\_82 & 5 & 18 & 3 & 3 & 3 & 3 & 3 & 27 & 6 & 3 & 6 \\ \hline
	decod24-v2\_43 & 4 & 22 & 0 & 0 & 0 & 0 & 9 & 15 & 0 & 0 & 0 \\ \hline
	decod24-v0\_38 & 4 & 23 & 0 & 0 & 0 & 0 & 9 & 15 & 9 & 0 & 0 \\ \hline
	miller\_11 & 3 & 23 & 0 & 0 & 0 & 0 & 6 & 9 & 0 & 0 & 0 \\ \hline
	alu-v3\_34 & 5 & 24 & 9 & 9 & 12 & 6 & 21 & 27 & 3 & 3 & 6 \\ \hline
	mod5d2\_64 & 5 & 25 & 15 & 9 & 18 & 9 & 27 & 36 & 18 & 12 & 12 \\ \hline
	4gt13-v1\_93 & 5 & 30 & 0 & 0 & 0 & 0 & 12 & 27 & 0 & 18 & 0 \\ \hline
	4gt13\_92 & 5 & 30 & 0 & 0 & 0 & 0 & 18 & 42 & 21 & 18 & 0 \\ \hline
	4mod5-bdd\_287 & 7 & 31 & 6 & 6 & 18 & 27 & 12 & 36 & 24 & 15 & 6 \\ \hline
	4mod5-v0\_18 & 5 & 31 & 6 & 6 & 9 & 15 & 27 & 36 & 15 & 9 & 9 \\ \hline
	one-two-three-v3\_101 & 5 & 32 & 9 & 9 & 9 & 9 & 27 & 36 & 18 & 12 & 9 \\ \hline
	one-two-three-v2\_100 & 5 & 32 & 9 & 9 & 9 & 9 & 9 & 30 & 24 & 21 & 15 \\ \hline
	decod24-bdd\_294 & 6 & 32 & 6 & 12 & 21 & 21 & 27 & 24 & 24 & 9 & 9 \\ \hline
	4mod5-v1\_23 & 5 & 32 & 6 & 6 & 12 & 21 & 27 & 36 & 24 & 15 & 6 \\ \hline
	rd32\_270 & 5 & 36 & 15 & 12 & 12 & 30 & 36 & 30 & 18 & 18 & 12 \\ \hline
	alu-bdd\_288 & 7 & 38 & 21 & 21 & 24 & 21 & 42 & 36 & 6 & 15 & 15 \\ \hline
	alu-v0\_26 & 5 & 38 & 12 & 12 & 30 & 9 & 24 & 36 & 27 & 45 & 24 \\ \hline
	decod24-v1\_41 & 5 & 38 & 3 & 3 & 3 & 12 & 24 & 45 & 39 & 21 & 9 \\ \hline
	4gt5\_75 & 5 & 38 & 9 & 9 & 33 & 12 & 27 & 51 & 3 & 18 & 15 \\ \hline
	4gt5\_76 & 5 & 46 & 15 & 15 & 21 & 15 & 18 & 48 & 33 & 27 & 15 \\ \hline
	4gt13\_91 & 5 & 49 & 6 & 6 & 6 & 6 & 15 & 45 & 21 & 6 & 15 \\ \hline
	alu-v4\_36 & 5 & 51 & 6 & 6 & 6 & 24 & 24 & 30 & 6 & 36 & 15 \\ \hline
	4gt13\_90 & 5 & 53 & 9 & 9 & 9 & 9 & 18 & 48 & 30 & 9 & 27 \\ \hline
	4gt5\_77 & 5 & 58 & 9 & 9 & 9 & 18 & 18 & 45 & 48 & 36 & 9 \\ \hline
	one-two-three-v1\_99 & 5 & 59 & 27 & 18 & 36 & 39 & 21 & 48 & 51 & 39 & 12 \\ \hline
	rd53\_138 & 8 & 60 & 30 & 18 & 45 & 30 & 51 & 42 & 48 & 39 & 27 \\ \hline
	decod24-v3\_45 & 5 & 64 & 15 & 15 & 15 & 24 & 27 & 66 & 54 & 39 & 15 \\ \hline
	one-two-three-v0\_98 & 5 & 65 & 27 & 18 & 21 & 36 & 33 & 63 & 27 & 27 & 24 \\ \hline
	4gt10-v1\_81 & 5 & 66 & 12 & 12 & 24 & 18 & 24 & 60 & 33 & 33 & 27 \\ \hline
	aj-e11\_165 & 5 & 69 & 33 & 18 & 42 & 30 & 21 & 33 & 30 & 24 & 18 \\ \hline
	alu-v2\_32 & 5 & 72 & 15 & 15 & 39 & 24 & 24 & 45 & 18 & 39 & 12 \\ \hline
	4mod7-v0\_94 & 5 & 72 & 12 & 12 & 12 & 18 & 24 & 51 & 48 & 42 & 18 \\ \hline
	4mod7-v1\_96 & 5 & 72 & 27 & 30 & 45 & 21 & 48 & 45 & 9 & 39 & 15 \\ \hline
	mod10\_176 & 5 & 78 & 15 & 15 & 15 & 24 & 42 & 66 & 15 & 36 & 24 \\ \hline
	4gt4-v0\_80 & 6 & 79 & 15 & 18 & 60 & 33 & 21 & 69 & 51 & 78 & 24 \\ \hline
	cnt3-5\_179 & 16 & 85 & 21 & 21 & 48 & 21 & 54 & 87 & 63 & 87 & 15 \\ \hline
	4gt12-v0\_88 & 6 & 86 & 21 & 30 & 45 & 24 & 57 & 66 & 15 & 21 & 21 \\ \hline
	ising\_model\_10 & 10 & 90 & 0 & 0 & 0 & 0 & 12 & 27 & 0 & 0 & 0 \\ \hline
	qft\_10 & 10 & 90 & 39 & 39 & 36 & 33 & 51 & 99 & 39 & 57 & 36 \\ \hline
	sys6-v0\_111 & 10 & 98 & 57 & 48 & 105 & 54 & 75 & 60 & 78 & 111 & 45 \\ \hline
	4\_49\_16 & 5 & 99 & 18 & 18 & 45 & 30 & 30 & 48 & 63 & 69 & 36 \\ \hline
	4gt12-v1\_89 & 6 & 100 & 18 & 18 & 39 & 30 & 24 & 81 & 72 & 93 & 24 \\ \hline
	0410184\_169 & 14 & 104 & 6 & 6 & 6 & 30 & 93 & 93 & 42 & 75 & 12 \\ \hline
	4gt4-v0\_79 & 6 & 105 & 12 & 9 & 12 & 12 & 30 & 87 & 48 & 96 & 12 \\ \hline
	hwb4\_49 & 5 & 107 & 42 & 51 & 48 & 42 & 48 & 63 & 54 & 45 & 33 \\ \hline
	mod10\_171 & 5 & 108 & 27 & 27 & 102 & 33 & 27 & 60 & 111 & 60 & 24 \\ \hline
	4gt4-v0\_78 & 6 & 109 & 15 & 12 & 15 & 15 & 33 & 93 & 60 & 99 & 15 \\ \hline
	4gt12-v0\_87 & 6 & 112 & 6 & 6 & 6 & 6 & 24 & 69 & 48 & 123 & 6 \\ \hline
	4gt4-v0\_72 & 6 & 113 & 21 & 27 & 72 & 33 & 51 & 84 & 51 & 90 & 42 \\ \hline
	4gt12-v0\_86 & 6 & 116 & 9 & 9 & 9 & 9 & 27 & 75 & 57 & 123 & 9 \\ \hline
	4gt4-v1\_74 & 6 & 119 & 36 & 27 & 48 & 30 & 96 & 93 & 24 & 114 & 78 \\ \hline
	ising\_model\_13 & 13 & 120 & 0 & 0 & 0 & 0 & 18 & 45 & 0 & 0 & 0 \\ \hline
	mini-alu\_167 & 5 & 126 & 30 & 36 & 69 & 33 & 57 & 87 & 87 & 75 & 33 \\ \hline
	one-two-three-v0\_97 & 5 & 128 & 42 & 42 & 39 & 72 & 66 & 90 & 54 & 66 & 66 \\ \hline
	rd53\_135 & 7 & 134 & 57 & 51 & 99 & 75 & 93 & 111 & 96 & 48 & 54 \\ \hline
	decod24-enable\_126 & 6 & 149 & 69 & 57 & 120 & 66 & 72 & 84 & 78 & 81 & 87 \\ \hline
	ham7\_104 & 7 & 149 & 39 & 39 & 54 & 36 & 78 & 51 & 48 & 102 & 81 \\ \hline
	ising\_model\_16 & 16 & 150 & 0 & 0 & 0 & 0 & 27 & 48 & 0 & 0 & 0 \\ \hline
	mod8-10\_178 & 6 & 152 & 48 & 30 & 114 & 33 & 36 & 87 & 120 & 162 & 21 \\ \hline
	rd84\_142 & 15 & 154 & 72 & 78 & 156 & 126 & 114 & 129 & 150 & 198 & 102 \\ \hline
	ex3\_229 & 6 & 175 & 36 & 24 & 21 & 51 & 63 & 102 & 144 & 174 & 18 \\ \hline
	4gt4-v0\_73 & 6 & 179 & 84 & 57 & 156 & 42 & 54 & 120 & 72 & 177 & 42 \\ \hline
	mod8-10\_177 & 6 & 196 & 60 & 48 & 183 & 54 & 84 & 87 & 162 & 135 & 39 \\ \hline
	alu-v2\_31 & 5 & 198 & 48 & 45 & 204 & 57 & 63 & 99 & 69 & 63 & 54 \\ \hline
	rd53\_131 & 7 & 200 & 57 & 42 & 165 & 78 & 78 & 81 & 132 & 87 & 90 \\ \hline
	C17\_204 & 7 & 205 & 72 & 63 & 183 & 75 & 93 & 147 & 204 & 114 & 96 \\ \hline
	alu-v2\_30 & 6 & 223 & 48 & 48 & 195 & 51 & 75 & 93 & 234 & 105 & 45 \\ \hline
	mod5adder\_127 & 6 & 239 & 75 & 72 & 162 & 78 & 81 & 117 & 132 & 87 & 51 \\ \hline
	qft\_16 & 16 & 240 & 153 & 153 & 174 & 135 & 201 & 249 & 228 & 195 & 135 \\ \hline
	rd53\_133 & 7 & 256 & 57 & 57 & 171 & 93 & 96 & 150 & 117 & 159 & 105 \\ \hline
	majority\_239 & 7 & 267 & 57 & 51 & 105 & 81 & 141 & 216 & 156 & 123 & 84 \\ \hline
	ex2\_227 & 7 & 275 & 102 & 81 & 147 & 93 & 108 & 126 & 234 & 270 & 96 \\ \hline
	cm82a\_208 & 8 & 283 & 78 & 72 & 225 & 99 & 102 & 228 & 222 & 222 & 84 \\ \hline
	sf\_276 & 6 & 336 & 30 & 30 & 24 & 30 & 111 & 159 & 336 & 381 & 24 \\ \hline
	sf\_274 & 6 & 336 & 141 & 42 & 270 & 30 & 51 & 180 & 237 & 384 & 24 \\ \hline
	con1\_216 & 9 & 415 & 177 & 114 & 438 & 147 & 189 & 195 & 306 & 375 & 192 \\ \hline
	rd53\_130 & 7 & 448 & 147 & 135 & 396 & 174 & 240 & 222 & 381 & 390 & 171 \\ \hline
	f2\_232 & 8 & 525 & 135 & 117 & 564 & 135 & 195 & 312 & 390 & 225 & 213 \\ \hline
	rd53\_251 & 8 & 564 & 156 & 156 & 510 & 159 & 234 & 240 & 588 & 309 & 204 \\ \hline
	hwb5\_53 & 6 & 598 & 195 & 162 & 255 & 240 & 195 & 222 & 390 & 210 & 174 \\ \hline
	z4\_268 & 11 & 1343 & 630 & 639 & 891 & 687 & 612 & 600 & 1332 & 1671 & 546 \\ \hline
	radd\_250 & 13 & 1405 & 555 & 633 & 1197 & 567 & 591 & 549 & 1350 & 1647 & 669 \\ \hline
	adr4\_197 & 13 & 1498 & 630 & 660 & 1158 & 714 & 579 & 675 & 1236 & 1146 & 711 \\ \hline
	sym6\_145 & 7 & 1701 & 513 & 465 & 1281 & 474 & 588 & 531 & 2025 & 2139 & 744 \\ \hline
	misex1\_241 & 15 & 2100 & 786 & 588 & 1566 & 726 & 825 & 735 & 2199 & 1263 & 921 \\ \hline
	rd73\_252 & 10 & 2319 & 1095 & 999 & 2220 & 822 & 1257 & 993 & 2370 & 2115 & 1065 \\ \hline
	cycle10\_2\_110 & 12 & 2648 & 1194 & 1152 & 2169 & 1347 & 1203 & 1179 & 2409 & 2424 & 1038 \\ \hline
	hwb6\_56 & 7 & 2952 & 1053 & 987 & 3144 & 1071 & 1182 & 1017 & 3015 & 1719 & 1104 \\ \hline
	square\_root\_7 & 15 & 3089 & 1338 & 1344 & 2508 & 1413 & 1377 & 1428 & 3087 & 1326 & 1353 \\ \hline
	sqn\_258 & 10 & 4459 & 1578 & 1503 & 3084 & 1896 & 1728 & 1917 & 4068 & 3192 & 1953 \\ \hline
	cm85a\_209 & 14 & 4986 & 2067 & 1986 & 4434 & 1929 & 2214 & 2151 & 4611 & 4173 & 2337 \\ \hline
	rd84\_253 & 12 & 5960 & 2352 & 2433 & 5361 & 2622 & 2634 & 2355 & 6429 & 5286 & 3198 \\ \hline
	root\_255 & 13 & 7493 & 3102 & 2553 & 6204 & 3546 & 3018 & 3222 & 7680 & 5601 & 3525 \\ \hline
	co14\_215 & 15 & 7840 & 4257 & 4245 & 8328 & 5091 & 4854 & 4038 & 9210 & 7752 & 4356 \\ \hline
	mlp4\_245 & 16 & 8232 & 3813 & 3912 & 7182 & 3933 & 4236 & 4128 & 8025 & 6462 & 4116 \\ \hline
	sym9\_148 & 10 & 9408 & 1884 & 1377 & 7080 & 1791 & 1971 & 2364 & 5370 & 6438 & 2172 \\ \hline
	urf2\_277 & 8 & 10066 & 6057 & 5640 & 10164 & 6054 & 6489 & 6303 & 10041 & 8205 & 5934 \\ \hline
	hwb7\_59 & 8 & 10681 & 3552 & 3009 & 7521 & 3696 & 3552 & 3465 & 10002 & 6378 & 4602 \\ \hline
	max46\_240 & 10 & 11844 & 3846 & 4065 & 11349 & 4527 & 5001 & 4143 & 11634 & 9681 & 5913 \\ \hline
	clip\_206 & 14 & 14772 & 7119 & 5880 & 13494 & 6372 & 7110 & 6513 & 16461 & 12624 & 6843 \\ \hline
	9symml\_195 & 11 & 15232 & 5589 & 4323 & 14100 & 5691 & 5811 & 5961 & 15351 & 11454 & 6036 \\ \hline
	sym9\_193 & 11 & 15232 & 5589 & 4323 & 14100 & 5691 & 5811 & 5961 & 15453 & 11454 & 6123 \\ \hline
	dist\_223 & 13 & 16624 & 7026 & 5352 & 14859 & 7227 & 7167 & 6099 & 18366 & 12834 & 6936 \\ \hline
	sao2\_257 & 14 & 16864 & 7521 & 7020 & 16863 & 7227 & 7533 & 7290 & 16365 & 11742 & 7827 \\ \hline
	urf5\_280 & 9 & 23764 & 11325 & 11526 & 22080 & 11841 & 11424 & 11691 & 25452 & 20436 & 13065 \\ \hline
	urf1\_278 & 9 & 26692 & 14754 & 13491 & 23544 & 14772 & 14088 & 14646 & 26121 & 24600 & 15678 \\ \hline
	sym10\_262 & 12 & 28084 & 9993 & 9708 & 26793 & 9999 & 11667 & 12978 & 32406 & 20115 & 11697 \\ \hline
	hwb8\_113 & 9 & 30372 & 11151 & 9144 & 25062 & 10878 & 12588 & 11442 & 31005 & 35376 & 14976 \\ \hline
	urf2\_152 & 8 & 35210 & 17814 & 15252 & 33774 & 18369 & 18306 & 18387 & 35910 & 25857 & 18342 \\ \hline 
	&&&&&&&&&&&\\
	sum & - & 333811 & 141252 & 126873 & 298017 & 144327 & 150108 & 149763 & 336021 & 272184 & 157056 \\ 
	max & 16  & 35210 & 17814 & 15252 & 33774 & 18369 & 18306 & 18387 & 35910	& 35376	& 18342  \\ 
	I-index & - & - & 1.4231 & {\bf 1.3801} & 1.8928 & 1.4324 & 1.4497 & 1.4486 & 2.0066 & 1.8154 & 1.4705 \\ \hline \\
\caption{Comparison on IBM Q Tokyo, where Q01x denotes the weakened combined Q0 and Q1-filters (cf. the last paragraph of Sec.~\ref{sec:eval} on page~\pageref{page:Q01x}), G and D denote \fidls-G and \fidls-D, respectively.  }
\label{tab:tokyo}
\end{longtable}
}
