# Supplementary material for: Qubit Mapping Based on Subgraph Isomorphism and Filtered Depth-Limited Search
Source: arXiv:2004.07138 source file (2021-09-22)
Supplement: Supplementary file 3 [file appendixB.tex]

{
\small

%\begin{tabular}[c]{@{}c@{}}Circuit\\   name\end{tabular} & 
%\begin{tabular}[c]{@{}c@{}}input \\ CNOT\end{tabular} & 
%\begin{tabular}[c]{@{}c@{}}tokyo\\ cambr.\end{tabular} & 
%\begin{tabular}[c]{@{}c@{}}topgr.\\ GQ12\end{tabular} &
%\begin{tabular}[c]{@{}c@{}}topgr.\\ GQ12x\end{tabular} & 
%\begin{tabular}[c]{@{}c@{}}topgr.\\ DQ12\end{tabular} & 
%\begin{tabular}[c]{@{}c@{}}wgtgr.\\ GQ12\end{tabular} & 
%\begin{tabular}[c]{@{}c@{}}empty\\ GQ12\end{tabular} & 
%\begin{tabular}[c]{@{}c@{}}naive\\ GQ12\end{tabular} & 
%\begin{tabular}[c]{@{}c@{}}\textsc{sabre}\\ added\end{tabular} &
%\begin{tabular}[c]{@{}c@{}}camb.\\ added\end{tabular} & 
%\begin{tabular}[c]{@{}c@{}}camb.\\ added\end{tabular} & 
%\begin{tabular}[c]{@{}c@{}}sahs.\\ added\end{tabular} \\ \hline

%\hline

%\endhead

 \begin{longtable}{ c*{10}{c|}c }
    \hline
     \multicolumn{2}{c|}{circ. info}
                         & tokyo 
                    & \multicolumn{3}{c|}{sycamore}
                    & \multicolumn{3}{c|}{rochester}
                    & \multicolumn{3}{c}{q19x19}\\
\hline	 

	name & \#CX & cambr. & G & D & cambr. & G & D & cambr. & G & D & cambr. 	
	\\ \hline

	ex1\_226 & 5 & 0 & 3 & 3 & 3 & 6 & 6 & 9 & 3 & 3 & 3 \\ \hline
	graycode6\_47 & 5 & 0 & 0 & 0 & 0 & 0 & 0 & 0 & 0 & 0 & 0 \\ \hline
	xor5\_254 & 5 & 0 & 3 & 3 & 3 & 6 & 6 & 9 & 3 & 3 & 3 \\ \hline
	ex-1\_166 & 9 & 0 & 9 & 9 & 9 & 9 & 9 & 9 & 9 & 9 & 9 \\ \hline
	4gt11\_84 & 9 & 0 & 9 & 9 & 9 & 9 & 9 & 9 & 9 & 9 & 9 \\ \hline
	4mod5-v0\_20 & 10 & 9 & 9 & 9 & 9 & 9 & 9 & 9 & 9 & 9 & 9 \\ \hline
	ham3\_102 & 11 & 9 & 9 & 9 & 9 & 9 & 9 & 9 & 9 & 12 & 9 \\ \hline
	4mod5-v1\_22 & 11 & 0 & 9 & 9 & 12 & 9 & 9 & 12 & 9 & 9 & 12 \\ \hline
	mod5d1\_63 & 13 & 0 & 21 & 18 & 12 & 18 & 18 & 18 & 18 & 18 & 12 \\ \hline
	4gt11\_83 & 14 & 12 & 9 & 9 & 15 & 18 & 15 & 18 & 9 & 9 & 9 \\ \hline
	rd32-v1\_68 & 16 & 9 & 18 & 18 & 18 & 21 & 21 & 24 & 21 & 21 & 18 \\ \hline
	rd32-v0\_66 & 16 & 12 & 18 & 18 & 18 & 24 & 21 & 24 & 21 & 21 & 21 \\ \hline
	4mod5-v1\_24 & 16 & 9 & 21 & 21 & 21 & 21 & 21 & 24 & 21 & 21 & 21 \\ \hline
	4mod5-v0\_19 & 16 & 0 & 18 & 18 & 18 & 18 & 18 & 21 & 18 & 18 & 18 \\ \hline
	mod5mils\_65 & 16 & 0 & 18 & 18 & 18 & 18 & 18 & 21 & 18 & 18 & 18 \\ \hline
	alu-v1\_29 & 17 & 0 & 27 & 27 & 18 & 18 & 18 & 18 & 24 & 24 & 18 \\ \hline
	alu-v2\_33 & 17 & 3 & 24 & 24 & 18 & 21 & 27 & 27 & 21 & 21 & 18 \\ \hline
	alu-v0\_27 & 17 & 3 & 27 & 27 & 18 & 21 & 27 & 27 & 24 & 24 & 18 \\ \hline
	3\_17\_13 & 17 & 9 & 18 & 18 & 18 & 18 & 21 & 24 & 18 & 18 & 18 \\ \hline
	alu-v1\_28 & 18 & 12 & 24 & 24 & 18 & 24 & 21 & 21 & 24 & 24 & 12 \\ \hline
	alu-v4\_37 & 18 & 3 & 27 & 27 & 18 & 21 & 27 & 27 & 24 & 24 & 18 \\ \hline
	alu-v3\_35 & 18 & 3 & 27 & 27 & 18 & 21 & 27 & 27 & 24 & 24 & 18 \\ \hline
	4gt11\_82 & 18 & 3 & 12 & 12 & 18 & 21 & 27 & 27 & 12 & 12 & 18 \\ \hline
	decod24-v2\_43 & 22 & 0 & 27 & 27 & 27 & 27 & 27 & 33 & 27 & 27 & 27 \\ \hline
	decod24-v0\_38 & 23 & 0 & 27 & 27 & 27 & 27 & 27 & 33 & 27 & 27 & 27 \\ \hline
	miller\_11 & 23 & 0 & 27 & 27 & 27 & 27 & 27 & 27 & 27 & 27 & 27 \\ \hline
	alu-v3\_34 & 24 & 3 & 30 & 30 & 33 & 36 & 33 & 45 & 30 & 30 & 33 \\ \hline
	mod5d2\_64 & 25 & 12 & 36 & 33 & 33 & 33 & 33 & 39 & 39 & 36 & 33 \\ \hline
	4gt13-v1\_93 & 30 & 18 & 36 & 36 & 36 & 51 & 48 & 45 & 39 & 36 & 36 \\ \hline
	4gt13\_92 & 30 & 18 & 39 & 36 & 36 & 42 & 39 & 51 & 36 & 36 & 36 \\ \hline
	4mod5-bdd\_287 & 31 & 15 & 42 & 42 & 45 & 42 & 42 & 63 & 39 & 36 & 42 \\ \hline
	4mod5-v0\_18 & 31 & 9 & 42 & 42 & 42 & 42 & 42 & 51 & 45 & 42 & 42 \\ \hline
	one-two-three-v3\_101 & 32 & 12 & 39 & 39 & 45 & 54 & 45 & 54 & 45 & 39 & 45 \\ \hline
	one-two-three-v2\_100 & 32 & 21 & 39 & 39 & 39 & 39 & 39 & 42 & 39 & 39 & 39 \\ \hline
	decod24-bdd\_294 & 32 & 9 & 39 & 39 & 36 & 54 & 48 & 48 & 39 & 39 & 36 \\ \hline
	4mod5-v1\_23 & 32 & 15 & 45 & 42 & 45 & 51 & 42 & 48 & 45 & 45 & 42 \\ \hline
	rd32\_270 & 36 & 18 & 57 & 54 & 48 & 57 & 54 & 66 & 54 & 51 & 48 \\ \hline
	alu-bdd\_288 & 38 & 15 & 63 & 54 & 48 & 78 & 60 & 63 & 60 & 54 & 48 \\ \hline
	alu-v0\_26 & 38 & 45 & 51 & 51 & 45 & 63 & 57 & 57 & 51 & 48 & 45 \\ \hline
	decod24-v1\_41 & 38 & 21 & 57 & 51 & 45 & 75 & 60 & 66 & 51 & 51 & 45 \\ \hline
	4gt5\_75 & 38 & 18 & 45 & 45 & 48 & 63 & 57 & 63 & 54 & 42 & 48 \\ \hline
	4gt5\_76 & 46 & 27 & 72 & 60 & 51 & 72 & 60 & 66 & 57 & 54 & 51 \\ \hline
	4gt13\_91 & 49 & 6 & 60 & 63 & 57 & 57 & 57 & 57 & 66 & 60 & 57 \\ \hline
	alu-v4\_36 & 51 & 36 & 69 & 72 & 60 & 72 & 72 & 78 & 72 & 63 & 60 \\ \hline
	4gt13\_90 & 53 & 9 & 63 & 69 & 60 & 60 & 60 & 60 & 69 & 63 & 60 \\ \hline
	4gt5\_77 & 58 & 36 & 87 & 78 & 66 & 90 & 81 & 105 & 78 & 81 & 66 \\ \hline
	one-two-three-v1\_99 & 59 & 39 & 84 & 78 & 75 & 102 & 102 & 108 & 84 & 78 & 75 \\ \hline
	rd53\_138 & 60 & 39 & 84 & 90 & 72 & 105 & 90 & 90 & 78 & 78 & 90 \\ \hline
	decod24-v3\_45 & 64 & 39 & 90 & 84 & 78 & 123 & 105 & 117 & 87 & 78 & 78 \\ \hline
	one-two-three-v0\_98 & 65 & 27 & 93 & 93 & 81 & 129 & 111 & 108 & 84 & 84 & 81 \\ \hline
	4gt10-v1\_81 & 66 & 33 & 87 & 87 & 90 & 123 & 108 & 114 & 93 & 90 & 90 \\ \hline
	aj-e11\_165 & 69 & 24 & 90 & 87 & 81 & 99 & 99 & 99 & 84 & 84 & 81 \\ \hline
	alu-v2\_32 & 72 & 39 & 99 & 96 & 90 & 117 & 117 & 117 & 96 & 93 & 90 \\ \hline
	4mod7-v0\_94 & 72 & 42 & 99 & 87 & 84 & 111 & 99 & 135 & 99 & 102 & 84 \\ \hline
	4mod7-v1\_96 & 72 & 39 & 96 & 90 & 105 & 102 & 102 & 111 & 123 & 111 & 105 \\ \hline
	mod10\_176 & 78 & 36 & 102 & 93 & 96 & 132 & 120 & 132 & 111 & 105 & 96 \\ \hline
	4gt4-v0\_80 & 79 & 78 & 114 & 114 & 117 & 138 & 129 & 141 & 138 & 117 & 117 \\ \hline
	cnt3-5\_179 & 85 & 87 & 153 & 153 & 129 & 195 & 261 & 141 & 168 & 138 & 150 \\ \hline
	4gt12-v0\_88 & 86 & 21 & 129 & 126 & 126 & 180 & 144 & 141 & 123 & 120 & 126 \\ \hline
	ising\_model\_10 & 90 & 0 & 0 & 0 & 0 & 0 & 0 & 0 & 0 & 0 & 27 \\ \hline
	qft\_10 & 90 & 57 & 63 & 72 & 75 & 108 & 108 & 147 & 66 & 75 & 72 \\ \hline
	sys6-v0\_111 & 98 & 111 & 138 & 159 & 144 & 192 & 159 & 171 & 141 & 138 & 147 \\ \hline
	4\_49\_16 & 99 & 69 & 138 & 123 & 120 & 186 & 159 & 171 & 141 & 135 & 120 \\ \hline
	4gt12-v1\_89 & 100 & 93 & 141 & 144 & 135 & 186 & 168 & 210 & 132 & 156 & 135 \\ \hline
	0410184\_169 & 104 & 75 & 141 & 144 & 135 & 354 & 195 & 210 & 135 & 129 & 138 \\ \hline
	4gt4-v0\_79 & 105 & 96 & 132 & 132 & 138 & 183 & 153 & 171 & 141 & 141 & 129 \\ \hline
	hwb4\_49 & 107 & 45 & 126 & 135 & 132 & 138 & 138 & 162 & 138 & 135 & 132 \\ \hline
	mod10\_171 & 108 & 60 & 162 & 156 & 135 & 174 & 174 & 195 & 162 & 159 & 135 \\ \hline
	4gt4-v0\_78 & 109 & 99 & 138 & 138 & 144 & 192 & 159 & 180 & 147 & 141 & 132 \\ \hline
	4gt12-v0\_87 & 112 & 123 & 147 & 147 & 150 & 186 & 162 & 174 & 156 & 141 & 135 \\ \hline
	4gt4-v0\_72 & 113 & 90 & 156 & 159 & 156 & 186 & 174 & 180 & 171 & 156 & 156 \\ \hline
	4gt12-v0\_86 & 116 & 123 & 156 & 150 & 150 & 192 & 168 & 177 & 159 & 144 & 138 \\ \hline
	4gt4-v1\_74 & 119 & 114 & 192 & 174 & 153 & 219 & 201 & 198 & 177 & 165 & 159 \\ \hline
	ising\_model\_13 & 120 & 0 & 0 & 0 & 0 & 0 & 0 & 0 & 0 & 0 & 0 \\ \hline
	mini-alu\_167 & 126 & 75 & 171 & 168 & 231 & 246 & 207 & 231 & 174 & 168 & 231 \\ \hline
	one-two-three-v0\_97 & 128 & 66 & 183 & 177 & 162 & 234 & 210 & 222 & 186 & 177 & 159 \\ \hline
	rd53\_135 & 134 & 48 & 201 & 183 & 174 & 270 & 228 & 264 & 210 & 189 & 180 \\ \hline
	decod24-enable\_126 & 149 & 81 & 222 & 213 & 189 & 288 & 228 & 243 & 216 & 207 & 189 \\ \hline
	ham7\_104 & 149 & 102 & 201 & 204 & 198 & 282 & 237 & 255 & 225 & 204 & 195 \\ \hline
	ising\_model\_16 & 150 & 0 & 0 & 0 & 0 & 0 & 0 & 30 & 0 & 0 & 24 \\ \hline
	mod8-10\_178 & 152 & 162 & 234 & 216 & 234 & 264 & 237 & 255 & 318 & 255 & 234 \\ \hline
	rd84\_142 & 154 & 198 & 231 & 237 & 228 & 300 & 291 & 327 & 228 & 234 & 267 \\ \hline
	ex3\_229 & 175 & 174 & 267 & 231 & 258 & 309 & 294 & 288 & 243 & 243 & 258 \\ \hline
	4gt4-v0\_73 & 179 & 177 & 246 & 231 & 213 & 327 & 315 & 339 & 261 & 246 & 213 \\ \hline
	mod8-10\_177 & 196 & 135 & 291 & 276 & 279 & 357 & 339 & 336 & 291 & 261 & 279 \\ \hline
	alu-v2\_31 & 198 & 63 & 294 & 306 & 273 & 321 & 300 & 306 & 300 & 297 & 273 \\ \hline
	rd53\_131 & 200 & 87 & 324 & 288 & 258 & 510 & 399 & 339 & 345 & 288 & 309 \\ \hline
	C17\_204 & 205 & 114 & 357 & 366 & 327 & 354 & 375 & 375 & 426 & 345 & 327 \\ \hline
	alu-v2\_30 & 223 & 105 & 327 & 327 & 288 & 468 & 420 & 447 & 312 & 306 & 279 \\ \hline
	mod5adder\_127 & 239 & 87 & 375 & 360 & 315 & 456 & 405 & 417 & 357 & 339 & 315 \\ \hline
	qft\_16 & 240 & 195 & 240 & 246 & 219 & 486 & 306 & 402 & 222 & 225 & 207 \\ \hline
	rd53\_133 & 256 & 159 & 372 & 363 & 330 & 555 & 462 & 447 & 438 & 366 & 378 \\ \hline
	majority\_239 & 267 & 123 & 402 & 378 & 387 & 486 & 444 & 483 & 396 & 387 & 369 \\ \hline
	ex2\_227 & 275 & 270 & 399 & 402 & 351 & 534 & 492 & 534 & 450 & 396 & 360 \\ \hline
	cm82a\_208 & 283 & 222 & 462 & 450 & 387 & 576 & 507 & 498 & 501 & 429 & 411 \\ \hline
	sf\_276 & 336 & 381 & 474 & 456 & 483 & 630 & 573 & 570 & 483 & 471 & 483 \\ \hline
	sf\_274 & 336 & 384 & 474 & 450 & 444 & 645 & 579 & 690 & 501 & 462 & 444 \\ \hline
	con1\_216 & 415 & 375 & 651 & 618 & 645 & 864 & 807 & 900 & 726 & 675 & 576 \\ \hline
	rd53\_130 & 448 & 390 & 672 & 639 & 588 & 903 & 813 & 858 & 753 & 738 & 639 \\ \hline
	f2\_232 & 525 & 225 & 813 & 768 & 762 & 1137 & 948 & 1002 & 837 & 774 & 744 \\ \hline
	rd53\_251 & 564 & 309 & 918 & 831 & 786 & 1146 & 981 & 1107 & 894 & 867 & 801 \\ \hline
	hwb5\_53 & 598 & 210 & 876 & 882 & 834 & 1137 & 1002 & 996 & 897 & 810 & 834 \\ \hline
	z4\_268 & 1343 & 1671 & 2259 & 2109 & 1917 & 3363 & 2691 & 2565 & 2286 & 2079 & 1989 \\ \hline
	radd\_250 & 1405 & 1647 & 2529 & 2313 & 2079 & 3102 & 2727 & 2808 & 2538 & 2271 & 2082 \\ \hline
	adr4\_197 & 1498 & 1146 & 2670 & 2328 & 2229 & 3741 & 3112 & 3060 & 2568 & 2511 & 2238 \\ \hline
	sym6\_145 & 1701 & 2139 & 2622 & 2445 & 2469 & 3285 & 2967 & 3204 & 2775 & 2532 & 2469 \\ \hline
	misex1\_241 & 2100 & 1263 & 3627 & 3396 & 3114 & 5241 & 4812 & 5154 & 3771 & 3330 & 3078 \\ \hline
	rd73\_252 & 2319 & 2115 & 4065 & 3774 & 3522 & 5454 & 4386 & 4704 & 3948 & 3612 & 3570 \\ \hline
	cycle10\_2\_110 & 2648 & 2424 & 4740 & 4332 & 4056 & 6549 & 6264 & 5994 & 4860 & 4320 & 3879 \\ \hline
	hwb6\_56 & 2952 & 1719 & 4455 & 4305 & 4296 & 5679 & 5196 & 5280 & 4680 & 4209 & 4296 \\ \hline
	square\_root\_7 & 3089 & 1326 & 6339 & 5433 & 4911 & 9028 & 8138 & 7488 & 6093 & 5691 & 4956 \\ \hline
	sqn\_258 & 4459 & 3192 & 7482 & 7068 & 6510 & 11595 & 9886 & 9183 & 8025 & 7041 & 6582 \\ \hline
	cm85a\_209 & 4986 & 4173 & 9033 & 8506 & 7431 & 12855 & 12214 & 9933 & 8901 & 8736 & 7650 \\ \hline
	rd84\_253 & 5960 & 5286 & 10875 & 10095 & 9315 & 16215 & 13036 & 12717 & 11391 & 10146 & 9156 \\ \hline
	root\_255 & 7493 & 5601 & 13473 & 12435 & 11634 & 18330 & 15927 & 15933 & 13947 & 13158 & 11757 \\ \hline
	co14\_215 & 7840 & 7752 & 16191 & 13995 & 12354 & 21966 & 20359 & 17205 & 17892 & 14632 & 13782 \\ \hline
	mlp4\_245 & 8232 & 6462 & 15090 & 13818 & 12738 & 21253 & 18046 & 18147 & 15651 & 14790 & 12999 \\ \hline
	sym9\_148 & 9408 & 6438 & 15594 & 14715 & 15219 & 22203 & 21050 & 19953 & 16323 & 16008 & 17325 \\ \hline
	urf2\_277 & 10066 & 8205 & 15780 & 15957 & 14178 & 23046 & 20439 & 22362 & 15894 & 15153 & 14118 \\ \hline
	hwb7\_59 & 10681 & 6378 & 16518 & 16329 & 15033 & 21960 & 19944 & 21642 & 16875 & 17730 & 15786 \\ \hline
	max46\_240 & 11844 & 9681 & 20271 & 19374 & 17994 & 30630 & 26661 & 22644 & 20793 & 19581 & 17472 \\ \hline
	clip\_206 & 14772 & 12624 & 27051 & 25287 & 24177 & 39030 & 35544 & 35277 & 29154 & 26180 & 23037 \\ \hline
	9symml\_195 & 15232 & 11454 & 27087 & 24894 & 23826 & 38608 & 34932 & 35325 & 27483 & 26055 & 23226 \\ \hline
	sym9\_193 & 15232 & 11454 & 27087 & 24894 & 23826 & 38608 & 34932 & 35325 & 27483 & 26055 & 23226 \\ \hline
	dist\_223 & 16624 & 12834 & 31323 & 28050 & 25467 & 42691 & 37538 & 38160 & 32202 & 28836 & 25605 \\ \hline
	sao2\_257 & 16864 & 11742 & 32490 & 28482 & 26472 & 44595 & 37950 & 37044 & 32760 & 29898 & 26283 \\ \hline
	urf5\_280 & 23764 & 20436 & 38466 & 36054 & 35304 & 53520 & 48080 & 49296 & 37860 & 40158 & 34206 \\ \hline
	urf1\_278 & 26692 & 24600 & 43518 & 41070 & 41217 & 84234 & 58130 & 69741 & 48567 & 45613 & 40209 \\ \hline
	sym10\_262 & 28084 & 20115 & 50592 & 46206 & 43917 & 77049 & 65813 & 62073 & 50673 & 46221 & 43653 \\ \hline
	hwb8\_113 & 30372 & 35376 & 48558 & 46611 & 46596 & 79506 & 58393 & 61218 & 48867 & 45411 & 46461 \\ \hline
	urf2\_152 & 35210 & 25857 & 54882 & 52659 & 51654 & 65868 & 61014 & 60837 & 58071 & 50925 & 48513 \\ \hline
	&&&&&&&&&&&\\
	sum/avg & 333811 & 272184 & 569946 & 531724 & 507606 & 829013 & 707779 & 713007 & 588192 & 547711 & 503901 \\
	max & 35210 & 35376 & 54882 & 52659 & 51654 & 84234 & 65813 & 69741 & 58071 & 50925 & 48513 \\ 
	I-index & - & 1.8154 & 2.7074 & 2.5929 & {\bf 2.5206} & 3.4835 & {\bf 3.1203} & 3.1360 & 2.7621 & 2.6408 & {\bf 2.5095} \\
\hline
\\
\caption{Comparison on the benchmark set $\mathcal{B}_c$, where G and D denote \fidls-G and \fidls-D, respectively.  }
\label{tab:b131-indices}
\end{longtable}
}
