# Supplementary material for: Qubit Mapping Based on Subgraph Isomorphism and Filtered Depth-Limited Search
Source: arXiv:2004.07138 source file (2021-09-22)
Supplement: Supplementary file 4 [file appendixC.tex]

{
\small
%\begin{longtable}{ccc|ccc|ccc|ccc}
%\hline
%\begin{tabular}[c]{@{}c@{}}Circuit\\   name\end{tabular} & 
%\begin{tabular}[c]{@{}c@{}}input \\ CNOT\end{tabular} & 
%\begin{tabular}[c]{@{}c@{}}tokyo\\ cambr.\end{tabular} & 
%\begin{tabular}[c]{@{}c@{}}topgr.\\ GQ12\end{tabular} &
%\begin{tabular}[c]{@{}c@{}}topgr.\\ GQ12x\end{tabular} & 
%\begin{tabular}[c]{@{}c@{}}topgr.\\ DQ12\end{tabular} & 
%\begin{tabular}[c]{@{}c@{}}wgtgr.\\ GQ12\end{tabular} & 
%\begin{tabular}[c]{@{}c@{}}empty\\ GQ12\end{tabular} & 
%\begin{tabular}[c]{@{}c@{}}naive\\ GQ12\end{tabular} & 
%\begin{tabular}[c]{@{}c@{}}\textsc{sabre}\\ added\end{tabular} &
%\begin{tabular}[c]{@{}c@{}}camb.\\ added\end{tabular} & 
%\begin{tabular}[c]{@{}c@{}}camb.\\ added\end{tabular} & 
%\begin{tabular}[c]{@{}c@{}}sahs.\\ added\end{tabular} \\ \hline

%\hline
 \begin{longtable}{ c*{10}{c|}c }
    \hline
     \multicolumn{3}{c|}{circ. info}
                    & \multicolumn{3}{c|}{Sycamore}
                    & \multicolumn{3}{c|}{Rochester}
                    & \multicolumn{3}{c}{Q19x19}\\
\hline	 
%	 &   &   & & sycamore  &  &  &rochester  &  &  & q19x19 & \\ 
	circ name & \#qubit & \#{\sc cnot}  & {\sc fidls-g} & {\sc fidls-d} & cambr. & {\sc fidls-g} & {\sc fidls-d} & cambr. & {\sc fidls-g} & {\sc fidls-d} & cambr. 
%\endhead
	
	\\ \hline

	\begin{tabular}[c]{@{}c@{}}
	H2\_cmplt\_JW\\ 
	\_ccpvdz
	\end{tabular}
	
	& 20 & 14616 & 1683 & 5694 & 1656 & 12021 & 7953 & 4137 & 6372 & 3609 & 5337 \\ \hline
	pf2\_30\_before & 30 & 360 & 0 & 0 & 123 & 384 & 225 & 177 & 0 & 0 & 249 \\ \hline
	pf4\_20\_before & 20 & 1200 & 0 & 0 & 261 & 0 & 0 & 339 & 0 & 0 & 519 \\ \hline
	pf1\_30\_before & 30 & 180 & 0 & 0 & 27 & 168 & 108 & 174 & 0 & 0 & 153 \\ \hline
	pf2\_20\_before & 20 & 240 & 0 & 0 & 687 & 0 & 0 & 984 & 0 & 0 & 1182 \\ \hline
	pf4\_30\_before & 30 & 1800 & 0 & 0 & 273 & 2391 & 1161 & 180 & 0 & 0 & 489 \\ \hline
	pf1\_20\_before & 20 & 120 & 0 & 0 & 195 & 0 & 0 & 249 & 0 & 0 & 231 \\ \hline
	pf1\_50\_after & 50 & 300 & 285 & 201 & 372 & 327 & 189 & 3684 & 132 & 87 & 3363 \\ \hline
	pf2\_40\_after & 40 & 1040 & 0 & 0 & 6711 & 0 & 0 & 7989 & 0 & 0 & 6918 \\ \hline
	 
	\begin{tabular}[c]{@{}c@{}}
	H2\_cmplt\_BK\\ 
    \_ccpvdz
    \end{tabular}
	
	& 20 & 11344 & 4104 & 5586 & 8442 & 13146 & 12669 & 20409 & 5556 & 9015 & 9075 \\ \hline
	LiH\_frz\_P\_631g & 20 & 13878 & 4725 & 8688 & 84 & 23283 & 11796 & 939 & 5619 & 4626 & 831 \\ \hline
	pf4\_20\_after & 20 & 2440 & 0 & 0 & 432 & 0 & 0 & 504 & 0 & 0 & 1329 \\ \hline
	pf2\_30\_after & 30 & 780 & 0 & 0 & 1353 & 966 & 687 & 2346 & 0 & 0 & 10434 \\ \hline
	pf2\_50\_before & 50 & 600 & 618 & 429 & 270 & 642 & 381 & 1794 & 267 & 192 & 1557 \\ \hline
	pf4\_30\_after & 30 & 3660 & 0 & 0 & 363 & 5262 & 3351 & 462 & 0 & 0 & 465 \\ \hline
	pf1\_40\_before & 40 & 240 & 0 & 0 & 1005 & 0 & 0 & 900 & 0 & 0 & 2457 \\ \hline
	pf2\_20\_after & 20 & 520 & 0 & 0 & 144 & 0 & 0 & 90 & 0 & 0 & 243 \\ \hline
	pf2\_50\_after & 50 & 1300 & 1368 & 966 & 489 & 1893 & 768 & 810 & 516 & 333 & 1356 \\ \hline
	pf2\_40\_before & 40 & 480 & 0 & 0 & 54 & 0 & 0 & 354 & 0 & 0 & 309 \\ \hline
	&&&&&&&&&&& \\
	sum & - & 55098 & 12783 & 21564 & 22941 & 60483 & 39288 & 46521 & 18462 & 17862 & 46497 \\ 
	max & 50 & 14616 & 4725 & 8688 & 8442 & 23283 & 12669 & 20409 & 6372 & 9015 & 10434 \\ 
	I-index & - & - & {\bf 1.2320} & 1.3914& 1.4164 & 2.0978 & {\bf 1.7131} & 1.8443 & 1.3351 & {\bf 1.3242} & 1.8439 \\ \hline \\

	\caption{Comparison on the benchmark set $\mathcal{B}_{bigQ}$ }
\label{tab:bigQ}
\end{longtable}
}

{
\small
%\begin{longtable}{ccc|cccc|cccc|cccc}
%\hline
%\begin{tabular}[c]{@{}c@{}}Circuit\\   name\end{tabular} & 
%\begin{tabular}[c]{@{}c@{}}input \\ CNOT\end{tabular} & 
%\begin{tabular}[c]{@{}c@{}}tokyo\\ cambr.\end{tabular} & 
%\begin{tabular}[c]{@{}c@{}}topgr.\\ GQ12\end{tabular} &
%\begin{tabular}[c]{@{}c@{}}topgr.\\ GQ12x\end{tabular} & 
%\begin{tabular}[c]{@{}c@{}}topgr.\\ DQ12\end{tabular} & 
%\begin{tabular}[c]{@{}c@{}}wgtgr.\\ GQ12\end{tabular} & 
%\begin{tabular}[c]{@{}c@{}}empty\\ GQ12\end{tabular} & 
%\begin{tabular}[c]{@{}c@{}}naive\\ GQ12\end{tabular} & 
%\begin{tabular}[c]{@{}c@{}}\textsc{sabre}\\ added\end{tabular} &
%\begin{tabular}[c]{@{}c@{}}camb.\\ added\end{tabular} & 
%\begin{tabular}[c]{@{}c@{}}camb.\\ added\end{tabular} & 
%\begin{tabular}[c]{@{}c@{}}sahs.\\ added\end{tabular} \\ \hline

%\hline
%\endhead
	
%\hline
%	 &  &  & syca. &  &  &  & roch. &  &  &  & 19x19 &  &  &  \\ \hline
	 
 \begin{longtable}{ cc*{12}{c|}c }
    \hline
     \multicolumn{3}{c|}{circ. info}
                    & \multicolumn{4}{c|}{mapp. \& search on Sycamore (s)}
                    & \multicolumn{4}{c|}{mapp. \& search on Rochester (s)}
                    & \multicolumn{4}{c}{mapp. \& search on Q19x19 (s)}\\
\hline	 
	 
	name & \#q & \#CX & mapp. & G & D & cam. & mapp. & G & D & cam. & mapp. & G & D & cam. \\ \hline
	\begin{tabular}[c]{@{}c@{}}
	H2\_cmplt\_JW\\ 
	\_ccpvdz
	\end{tabular} 
	
	& 20 & 14616 & 38.1 & 113 & 54.7 & 0.2 & 34.7 & 213 & 66.4 & 0.2 & 34.6 & 198 & 65.3 & 28 \\ \hline
	pf2\_30\_before & 30 & 360 & 233 & 0.01 & 0.01 & 0.1 & 4.8 & 0.17 & 0.11 & 0.1 & 0.4 & 0.01 & 0.02 & 26.8 \\ \hline
	pf4\_20\_before & 20 & 1200 & 1.7 & 0.02 & 0.02 & 0.1 & 0.1 & 0.02 & 0.02 & 0.1 & 0.8 & 0.04 & 0.04 & 27 \\ \hline
	pf1\_30\_before & 30 & 180 & 237 & 0 & 0 & 0.1 & 4.8 & 0.08 & 0.05 & 0.1 & 0.3 & 0.01 & 0.01 & 26.6 \\ \hline
	pf2\_20\_before & 20 & 240 & 1.9 & 0.01 & 0 & 0.2 & 0.1 & 0 & 0 & 0.2 & 0.8 & 0.01 & 0.01 & 27.3 \\ \hline
	pf4\_30\_before & 30 & 1800 & 235 & 0.05 & 0.05 & 0.1 & 4.90 & 1.06 & 0.67 & 0.1 & 0.3 & 0.08 & 0.07 & 26.7 \\ \hline
	pf1\_20\_before & 20 & 120 & 2.4 & 0 & 0 & 0.1 & 0 & 0 & 0 & 0.1 & 0.8 & 0 & 0 & 26.9 \\ \hline
	pf1\_50\_after & 50 & 300 & 224 & 2.15 & 0.7 & 0.1 & 6.8 & 1.45 & 0.45 & 0.2 & 305 & 1.09 & 1.01 & 27.2 \\ \hline
	pf2\_40\_after & 40 & 1040 & 0.3 & 0.04 & 0.04 & 0.3 & 0.7 & 0.04 & 0.04 & 0.4 & 17.10 & 0.06 & 0.07 & 28.2 \\ \hline
	\begin{tabular}[c]{@{}c@{}}
	H2\_cmplt\_BK\\ 
    \_ccpvdz
    \end{tabular}
	
	& 20 & 11344 & 24.9 & 300 & 69.3 & 0.3 & 24.3 & 234 & 109 & 0.5 & 24.1 & 260 & 129 & 29.5 \\ \hline
	LiH\_frz\_P\_631g & 20 & 13878 & 225 & 268 & 78.9 & 0.1 & 24.7 & 254 & 87.6 & 0.1 & 225 & 248 & 70.7 & 26.5 \\ \hline
	pf4\_20\_after & 20 & 2440 & 1.9 & 0.05 & 0.05 & 0.1 & 0.1 & 0.05 & 0.05 & 0.1 & 0.8 & 0.09 & 0.08 & 26.8 \\ \hline
	pf2\_30\_after & 30 & 780 & 232 & 0.02 & 0.02 & 0.3 & 4.8 & 0.73 & 0.54 & 0.3 & 0.2 & 0.03 & 0.03 & 29.3  \\ \hline
	pf2\_50\_before & 50 & 600 & 221 & 1.32 & 1.79 & 0.1 & 6.8 & 1.38 & 1.17 & 0.1 & 304 & 1.4 & 1.74 & 26.6  \\ \hline
	pf4\_30\_after & 30 & 3660 & 231 & 0.12 & 0.12 & 0.1 & 5 & 4.93 & 3.03 & 0.1 & 0.2 & 0.18 & 0.16 & 26.7  \\ \hline
	pf1\_40\_before & 40 & 240 & 0.2 & 0.01 & 0.01 & 0.1 & 0.7 & 0.01 & 0.01 & 0.1 & 16.9 & 0.01 & 0.01 & 26.9  \\ \hline
	pf2\_20\_after & 20 & 520 & 1.8 & 0.01 & 0.01 & 0.1 & 0.1 & 0.01 & 0.01 & 0.1 & 0.8 & 0.02 & 0.02 & 26.3  \\ \hline
	pf2\_50\_after & 50 & 1300 & 220 & 5.89 & 2.58 & 0.1 & 7.1 & 3.01 & 1.91 & 0.1 & 305 & 5.64 & 4.23 & 27  \\ \hline
	pf2\_40\_before & 40 & 480 & 0.2 & 0.02 & 0.02 & 0.1 & 0.7 & 0.02 & 0.02 & 0.1 & 17.4 & 0.02 & 0.02 & 26.3  \\ \hline
	 &  &  &  &  &  &  &  &  &  &  & & & &    \\ 
	 sum & - & 55098 & 2131 & 691 & 208 & 2.54 & 131 & 714 & 271 & 2.99 & 1254 & 715 & 272 & 517  \\ 
	max & 50 & 14616 & 237 & 300 & 78.9 & 0.35 & 34.7 & 254 & 109 & 0.5 & 305 & 260 & 129 & 29.5 \\ 
 \hline
	\\
\caption{Comparison on the benchmark set $\mathcal{B}_{bigQ}$: Time, where columns $G$ ($D$, cam., resp.) denote the search time of $\fidls$-$G$ ($\fidls$-$D$, the Cambridge algorithm, resp.) on the corresponding devices, columns mapp. denote the topgraph initial mapping construction time on the corresponding devices}
\label{tab:bigQtime}
\end{longtable}
}
