# Supplementary material for: Qubit Mapping Based on Subgraph Isomorphism and Filtered Depth-Limited Search
Source: arXiv:2004.07138 source file (2021-09-22)
Supplement: Supplementary file 5 [file appendixD.tex]

{
\small
%\begin{longtable}{ccc|cccccccc}

%\begin{tabular}{| *{11}{c|} }
 \begin{longtable}{cc *{8}{c|}c }
    \hline
     \multicolumn{3}{c|}{circ. info}
                    & \multicolumn{5}{c|}{mapping \& search on Q Tokyo (s)}
                           & \multicolumn{3}{c}{mapp. \& search on Q19x19 (s)}  \\
\hline
	circ name & \#q & \#CX & mapp. & G & GQ01x & Cambr. & SABRE & mapp. & D  & Cambr. \\ \hline
	ex1\_226 & 6 & 5 & 0.1 & 0 & 0 & 0 & 0 & 0.1 & 0.09 & 26.33 \\ \hline
	graycode6\_47 & 6 & 5 & 0.1 & 0 & 0 & 0 & 0 & 0.2 & 0 & 26.22 \\ \hline
	xor5\_254 & 6 & 5 & 0.1 & 0 & 0 & 0 & 0 & 0.1 & 0.1 & 26.81 \\ \hline
	ex-1\_166 & 3 & 9 & 0.1 & 0 & 0 & 0 & 0 & 0.1 & 0.03 & 27.45 \\ \hline
	4gt11\_84 & 4 & 9 & 0.1 & 0 & 0 & 0 & 0 & 0.1 & 0.11 & 26.51 \\ \hline
	4mod5-v0\_20 & 5 & 10 & 0.1 & 0 & 0 & 0 & 0.01 & 0.1 & 0.05 & 28.42 \\ \hline
	ham3\_102 & 3 & 11 & 0.1 & 0 & 0 & 0 & 0.01 & 0.1 & 0.04 & 30.14 \\ \hline
	4mod5-v1\_22 & 5 & 11 & 0.1 & 0 & 0 & 0 & 0 & 0.1 & 0.06 & 26.14 \\ \hline
	mod5d1\_63 & 5 & 13 & 0.1 & 0 & 0 & 0 & 0.01 & 0.1 & 0.09 & 29.72 \\ \hline
	4gt11\_83 & 5 & 14 & 0.1 & 0 & 0 & 0 & 0.01 & 0.1 & 0.03 & 27.19 \\ \hline
	rd32-v1\_68 & 4 & 16 & 0.1 & 0 & 0 & 0 & 0.01 & 0.1 & 0.13 & 30.23 \\ \hline
	rd32-v0\_66 & 4 & 16 & 0.1 & 0 & 0 & 0 & 0.01 & 0.1 & 0.13 & 28.76 \\ \hline
	4mod5-v1\_24 & 5 & 16 & 0.1 & 0 & 0 & 0 & 0.01 & 0.1 & 0.11 & 27.88 \\ \hline
	4mod5-v0\_19 & 5 & 16 & 0.1 & 0 & 0 & 0 & 0.01 & 0.1 & 0.2 & 26.27 \\ \hline
	mod5mils\_65 & 5 & 16 & 0.1 & 0 & 0 & 0 & 0.01 & 0.1 & 0.19 & 26.3 \\ \hline
	alu-v1\_29 & 5 & 17 & 0.1 & 0.07 & 0.21 & 0 & 0.01 & 0.1 & 0.22 & 25.96 \\ \hline
	alu-v2\_33 & 5 & 17 & 0.1 & 0.04 & 0.1 & 0 & 0.01 & 0.1 & 0.15 & 31.19 \\ \hline
	alu-v0\_27 & 5 & 17 & 0.1 & 0.07 & 0.17 & 0 & 0.01 & 0.1 & 0.23 & 30.85 \\ \hline
	3\_17\_13 & 3 & 17 & 0.1 & 0 & 0 & 0 & 0.01 & 0.1 & 0.06 & 28.22 \\ \hline
	alu-v1\_28 & 5 & 18 & 0.1 & 0.07 & 0.08 & 0 & 0.01 & 0.1 & 0.19 & 26.39 \\ \hline
	alu-v4\_37 & 5 & 18 & 0.1 & 0.04 & 0.08 & 0 & 0.01 & 0.1 & 0.23 & 29.82 \\ \hline
	alu-v3\_35 & 5 & 18 & 0.1 & 0.03 & 0.08 & 0 & 0.01 & 0.1 & 0.22 & 28.44 \\ \hline
	4gt11\_82 & 5 & 18 & 0.1 & 0.04 & 0.08 & 0 & 0.01 & 0.1 & 0.04 & 28.7 \\ \hline
	decod24-v2\_43 & 4 & 22 & 0.1 & 0 & 0 & 0 & 0.01 & 0.1 & 0.16 & 26.6 \\ \hline
	decod24-v0\_38 & 4 & 23 & 0.1 & 0 & 0 & 0 & 0.01 & 0.1 & 0.16 & 26.4 \\ \hline
	miller\_11 & 3 & 23 & 0.1 & 0 & 0 & 0 & 0.01 & 0.1 & 0.09 & 26.02 \\ \hline
	alu-v3\_34 & 5 & 24 & 0.1 & 0.04 & 0.11 & 0 & 0.01 & 0.1 & 0.23 & 28.54 \\ \hline
	mod5d2\_64 & 5 & 25 & 0 & 0.04 & 0.08 & 0 & 0.01 & 0.1 & 0.32 & 28.65 \\ \hline
	4gt13-v1\_93 & 5 & 30 & 0.1 & 0 & 0 & 0 & 0.02 & 0.1 & 0.22 & 28.9 \\ \hline
	4gt13\_92 & 5 & 30 & 0.1 & 0 & 0 & 0 & 0.02 & 0.1 & 0.16 & 28.75 \\ \hline
	4mod5-bdd\_287 & 7 & 31 & 0.1 & 0.02 & 0.05 & 0 & 0.02 & 0.1 & 0.35 & 29.07 \\ \hline
	4mod5-v0\_18 & 5 & 31 & 0.1 & 0.02 & 0.04 & 0 & 0.02 & 0.1 & 0.39 & 30.26 \\ \hline
	one-two-three-v3\_101 & 5 & 32 & 0 & 0.02 & 0.03 & 0 & 0.02 & 0.1 & 0.29 & 29.69 \\ \hline
	one-two-three-v2\_100 & 5 & 32 & 0.1 & 0.03 & 0.03 & 0 & 0.02 & 0.1 & 0.26 & 26.97 \\ \hline
	decod24-bdd\_294 & 6 & 32 & 0 & 0.05 & 0.23 & 0 & 0.02 & 0.1 & 0.28 & 26.58 \\ \hline
	4mod5-v1\_23 & 5 & 32 & 0.1 & 0.02 & 0.04 & 0 & 0.02 & 0.1 & 0.38 & 26.44 \\ \hline
	rd32\_270 & 5 & 36 & 0 & 0.04 & 0.08 & 0 & 0.02 & 0.1 & 0.44 & 26.25 \\ \hline
	alu-bdd\_288 & 7 & 38 & 0.1 & 0.09 & 0.17 & 0 & 0.02 & 0.1 & 0.39 & 28.57 \\ \hline
	alu-v0\_26 & 5 & 38 & 0.1 & 0.05 & 0.15 & 0 & 0.03 & 0.1 & 0.32 & 29.99 \\ \hline
	decod24-v1\_41 & 5 & 38 & 0 & 0.02 & 0.05 & 0 & 0.03 & 0.1 & 0.28 & 30.57 \\ \hline
	4gt5\_75 & 5 & 38 & 0 & 0.04 & 0.09 & 0 & 0.02 & 0.1 & 0.22 & 26.33 \\ \hline
	4gt5\_76 & 5 & 46 & 0 & 0.1 & 0.15 & 0 & 0.03 & 0.1 & 0.4 & 29.95 \\ \hline
	4gt13\_91 & 5 & 49 & 0 & 0.03 & 0.07 & 0 & 0.03 & 0.1 & 0.6 & 29.11 \\ \hline
	alu-v4\_36 & 5 & 51 & 0 & 0.02 & 0.04 & 0 & 0.02 & 0.1 & 0.36 & 29.34 \\ \hline
	4gt13\_90 & 5 & 53 & 0 & 0.05 & 0.13 & 0 & 0.02 & 0.1 & 0.71 & 29.09 \\ \hline
	4gt5\_77 & 5 & 58 & 0.1 & 0.1 & 0.58 & 0 & 0.05 & 0.1 & 0.6 & 29.43 \\ \hline
	one-two-three-v1\_99 & 5 & 59 & 0 & 0.09 & 0.16 & 0 & 0.04 & 0.1 & 0.52 & 26.68 \\ \hline
	rd53\_138 & 8 & 60 & 0.1 & 0.46 & 0.29 & 0 & 0.04 & 0.1 & 1.49 & 29.74 \\ \hline
	decod24-v3\_45 & 5 & 64 & 0.1 & 0.12 & 0.64 & 0 & 0.04 & 0.1 & 0.45 & 27.43 \\ \hline
	one-two-three-v0\_98 & 5 & 65 & 0 & 0.14 & 0.22 & 0 & 0.03 & 0.1 & 0.56 & 27.05 \\ \hline
	4gt10-v1\_81 & 5 & 66 & 0.1 & 0.1 & 0.59 & 0 & 0.04 & 0.1 & 0.53 & 26.41 \\ \hline
	aj-e11\_165 & 5 & 69 & 0 & 0.12 & 0.14 & 0 & 0.03 & 0.1 & 0.56 & 30.47 \\ \hline
	alu-v2\_32 & 5 & 72 & 0 & 0.1 & 0.17 & 0 & 0.03 & 0.1 & 0.51 & 29.52 \\ \hline
	4mod7-v0\_94 & 5 & 72 & 0.1 & 0.12 & 0.47 & 0 & 0.04 & 0.1 & 0.73 & 30.49 \\ \hline
	4mod7-v1\_96 & 5 & 72 & 0 & 0.07 & 0.23 & 0 & 0.03 & 0.1 & 0.95 & 29.83 \\ \hline
	mod10\_176 & 5 & 78 & 0 & 0.1 & 0.23 & 0 & 0.03 & 0.1 & 0.76 & 28.09 \\ \hline
	4gt4-v0\_80 & 6 & 79 & 0.1 & 0.04 & 0.27 & 0 & 0.05 & 0.1 & 0.82 & 28.27 \\ \hline
	cnt3-5\_179 & 16 & 85 & 0.2 & 0.25 & 0.56 & 0 & 0.08 & 0.2 & 10.38 & 27.35 \\ \hline
	4gt12-v0\_88 & 6 & 86 & 0 & 0.13 & 0.2 & 0 & 0.04 & 0.1 & 0.94 & 29.22 \\ \hline
	ising\_model\_10 & 10 & 90 & 0.1 & 0 & 0 & 0 & 0.03 & 0.2 & 0 & 26.04 \\ \hline
	qft\_10 & 10 & 90 & 0 & 1.6 & 1.6 & 0 & 0.05 & 0.1 & 7.72 & 26.4 \\ \hline
	sys6-v0\_111 & 10 & 98 & 0.1 & 1.39 & 1.78 & 0 & 0.06 & 0.1 & 3.72 & 26.44 \\ \hline
	4\_49\_16 & 5 & 99 & 0.1 & 0.1 & 0.41 & 0 & 0.05 & 0.1 & 0.95 & 26.22 \\ \hline
	4gt12-v1\_89 & 6 & 100 & 0.1 & 0.12 & 0.47 & 0 & 0.07 & 0.1 & 1.2 & 28.53 \\ \hline
	0410184\_169 & 14 & 104 & 13 & 0.04 & 0.06 & 0 & 0.08 & 0.4 & 1.61 & 25.69 \\ \hline
	4gt4-v0\_79 & 6 & 105 & 0 & 0.12 & 0.78 & 0 & 0.06 & 0.1 & 1.06 & 28.34 \\ \hline
	hwb4\_49 & 5 & 107 & 0 & 0.15 & 0.31 & 0 & 0.07 & 0.1 & 1 & 26.3 \\ \hline
	mod10\_171 & 5 & 108 & 0 & 0.22 & 0.8 & 0 & 0.06 & 0.1 & 1.19 & 26.73 \\ \hline
	4gt4-v0\_78 & 6 & 109 & 0 & 0.13 & 0.84 & 0 & 0.07 & 0.1 & 1.03 & 28.16 \\ \hline
	4gt12-v0\_87 & 6 & 112 & 0 & 0.03 & 0.07 & 0 & 0.06 & 0.1 & 1.15 & 28.45 \\ \hline
	4gt4-v0\_72 & 6 & 113 & 0 & 0.41 & 0.24 & 0 & 0.06 & 0.1 & 1.22 & 28.41 \\ \hline
	4gt12-v0\_86 & 6 & 116 & 0 & 0.05 & 0.11 & 0 & 0.06 & 0.1 & 1.16 & 28.46 \\ \hline
	4gt4-v1\_74 & 6 & 119 & 0 & 0.15 & 0.29 & 0 & 0.07 & 0.1 & 1.22 & 27.87 \\ \hline
	ising\_model\_13 & 13 & 120 & 0.1 & 0 & 0 & 0 & 0.04 & 0.2 & 0 & 26.48 \\ \hline
	mini-alu\_167 & 5 & 126 & 0 & 0.3 & 1.23 & 0 & 0.08 & 0.1 & 2.62 & 26.23 \\ \hline
	one-two-three-v0\_97 & 5 & 128 & 0 & 0.2 & 0.43 & 0 & 0.07 & 0.1 & 1.31 & 27.2 \\ \hline
	rd53\_135 & 7 & 134 & 0 & 0.52 & 1.54 & 0 & 0.08 & 0.1 & 1.9 & 29.64 \\ \hline
	decod24-enable\_126 & 6 & 149 & 0 & 0.29 & 0.3 & 0 & 0.09 & 0.1 & 1.82 & 26.41 \\ \hline
	ham7\_104 & 7 & 149 & 0 & 0.45 & 0.66 & 0 & 0.09 & 0.1 & 1.36 & 26.16 \\ \hline
	ising\_model\_16 & 16 & 150 & 0.1 & 0 & 0 & 0 & 0.05 & 0.2 & 0 & 26.34 \\ \hline
	mod8-10\_178 & 6 & 152 & 0 & 0.18 & 0.73 & 0 & 0.1 & 0.1 & 2.06 & 27.48 \\ \hline
	rd84\_142 & 15 & 154 & 4.5 & 5.01 & 8.94 & 0 & 0.12 & 0.1 & 8.19 & 28.49 \\ \hline
	ex3\_229 & 6 & 175 & 0.1 & 0.16 & 0.31 & 0 & 0.11 & 0.1 & 1.7 & 26.14 \\ \hline
	4gt4-v0\_73 & 6 & 179 & 0 & 0.25 & 0.47 & 0 & 0.1 & 0.1 & 2.15 & 28.56 \\ \hline
	mod8-10\_177 & 6 & 196 & 0 & 0.22 & 0.52 & 0 & 0.11 & 0.1 & 2 & 27.6 \\ \hline
	alu-v2\_31 & 5 & 198 & 0 & 0.22 & 0.57 & 0 & 0.1 & 0.1 & 2.32 & 30.51 \\ \hline
	rd53\_131 & 7 & 200 & 0.1 & 0.41 & 0.99 & 0 & 0.13 & 0.1 & 1.76 & 26.28 \\ \hline
	C17\_204 & 7 & 205 & 0.1 & 0.46 & 1.2 & 0 & 0.15 & 0.1 & 2.78 & 28.33 \\ \hline
	alu-v2\_30 & 6 & 223 & 0.1 & 0.25 & 0.69 & 0 & 0.14 & 0.1 & 2.1 & 31.11 \\ \hline
	mod5adder\_127 & 6 & 239 & 0 & 0.96 & 2.51 & 0 & 0.15 & 0.1 & 2.96 & 29.33 \\ \hline
	qft\_16 & 16 & 240 & 0.1 & 21.06 & 19.72 & 0.01 & 0.26 & 0.1 & 29.84 & 26.46 \\ \hline
	rd53\_133 & 7 & 256 & 0.2 & 0.39 & 1.6 & 0 & 0.17 & 0.1 & 2.6 & 27.89 \\ \hline
	majority\_239 & 7 & 267 & 0.5 & 0.47 & 1.48 & 0 & 0.19 & 0.1 & 3.28 & 26.67 \\ \hline
	ex2\_227 & 7 & 275 & 0.1 & 0.41 & 2.66 & 0 & 0.21 & 0.1 & 3.56 & 26.32 \\ \hline
	cm82a\_208 & 8 & 283 & 0.2 & 0.75 & 2.18 & 0 & 0.2 & 0.1 & 6.31 & 28.1 \\ \hline
	sf\_276 & 6 & 336 & 0 & 0.16 & 0.66 & 0 & 0.27 & 0.1 & 4.22 & 27.92 \\ \hline
	sf\_274 & 6 & 336 & 0.1 & 1.09 & 0.67 & 0.01 & 0.24 & 0.1 & 3.3 & 27.92 \\ \hline
	con1\_216 & 9 & 415 & 0.1 & 2.24 & 6.21 & 0.01 & 0.33 & 0.1 & 7.97 & 27.27 \\ \hline
	rd53\_130 & 7 & 448 & 0.1 & 0.98 & 4.38 & 0.01 & 0.37 & 0.1 & 7.26 & 26.35 \\ \hline
	f2\_232 & 8 & 525 & 0.1 & 0.79 & 2.18 & 0.01 & 0.46 & 0.1 & 7.75 & 26.3 \\ \hline
	rd53\_251 & 8 & 564 & 0.1 & 1.36 & 3.85 & 0.01 & 0.56 & 0.1 & 6.06 & 30.37 \\ \hline
	hwb5\_53 & 6 & 598 & 0.4 & 1.49 & 4.61 & 0.01 & 0.55 & 0.1 & 6.94 & 26.32 \\ \hline
	z4\_268 & 11 & 1343 & 0.2 & 16.19 & 68.62 & 0.02 & 1.95 & 0.2 & 23.89 & 27.4 \\ \hline
	radd\_250 & 13 & 1405 & 0.5 & 28.21 & 133.9 & 0.03 & 2.31 & 0.5 & 28.15 & 27.02 \\ \hline
	adr4\_197 & 13 & 1498 & 0.5 & 19.85 & 81.32 & 0.03 & 2.92 & 0.4 & 36.17 & 31.86 \\ \hline
	sym6\_145 & 7 & 1701 & 0.1 & 2.93 & 10.16 & 0.02 & 3.03 & 0.1 & 18.98 & 29.54 \\ \hline
	misex1\_241 & 15 & 2100 & 0.7 & 24.62 & 48.27 & 0.03 & 3.71 & 0.6 & 30.53 & 26.83 \\ \hline
	rd73\_252 & 10 & 2319 & 0.1 & 9.72 & 46.69 & 0.04 & 4.42 & 0.2 & 37.86 & 30.41 \\ \hline
	cycle10\_2\_110 & 12 & 2648 & 0.4 & 10.93 & 98.09 & 0.05 & 6.94 & 0.3 & 39.69 & 28.37 \\ \hline
	hwb6\_56 & 7 & 2952 & 0.1 & 8.67 & 31.94 & 0.03 & 8.1 & 0.2 & 33.13 & 27.11 \\ \hline
	square\_root\_7 & 15 & 3089 & 0.5 & 228.29 & 622.04 & 0.04 & 8.70 & 0.9 & 88.39 & 31.7 \\ \hline
	sqn\_258 & 10 & 4459 & 0.4 & 17.73 & 80.05 & 0.06 & 16.89 & 0.4 & 82.07 & 29.99 \\ \hline
	cm85a\_209 & 14 & 4986 & 15.4 & 37.38 & 165.1 & 0.12 & 21.38 & 0.8 & 84.71 & 30.98 \\ \hline
	rd84\_253 & 12 & 5960 & 0.9 & 54.35 & 259.90 & 0.11 & 20.6 & 0.8 & 121.22 & 32.37 \\ \hline
	root\_255 & 13 & 7493 & 1.5 & 108.25 & 431.08 & 0.13 & 43.27 & 1.5 & 176.86 & 32.30 \\ \hline
	co14\_215 & 15 & 7840 & 3.3 & 128.33 & 902.44 & 0.16 & 39.08 & 0.6 & 348.37 & 32.28 \\ \hline
	mlp4\_245 & 16 & 8232 & 4.90 & 369.4 & 1515.64 & 0.17 & 43.19 & 5.2 & 201.5 & 31.67 \\ \hline
	sym9\_148 & 10 & 9408 & 1.4 & 30.81 & 86.34 & 0.12 & 66.7 & 1.10 & 136.9 & 33.58 \\ \hline
	urf2\_277 & 8 & 10066 & 0.5 & 130.97 & 246.29 & 0.11 & 82.41 & 0.6 & 168.99 & 33.45 \\ \hline
	hwb7\_59 & 8 & 10681 & 0.6 & 37.59 & 136.54 & 0.11 & 89.33 & 0.6 & 127.54 & 30.74 \\ \hline
	max46\_240 & 10 & 11844 & 0.9 & 50.16 & 230.62 & 0.15 & 121.61 & 0.7 & 239.07 & 32.16 \\ \hline
	clip\_206 & 14 & 14772 & 6.5 & 263.67 & 1177.78 & 0.38 & 141.4 & 2.20 & 357.91 & 36.96 \\ \hline
	9symml\_195 & 11 & 15232 & 0.7 & 77.2 & 309.4 & 0.29 & 186.31 & 0.8 & 264.68 & 39.34 \\ \hline
	sym9\_193 & 11 & 15232 & 0.7 & 70.29 & 331.11 & 0.24 & 184.7 & 0.7 & 270.6 & 37.99 \\ \hline
	dist\_223 & 13 & 16624 & 1.9 & 303.9 & 785.18 & 0.29 & 210.59 & 2.1 & 429.33 & 36 \\ \hline
	sao2\_257 & 14 & 16864 & 2.7 & 503.45 & 1412.92 & 0.3 & 212.71 & 2.7 & 510.42 & 39.17 \\ \hline
	urf5\_280 & 9 & 23764 & 0.7 & 272.75 & 682.58 & 0.32 & 441.97 & 0.7 & 412.79 & 39.9 \\ \hline
	urf1\_278 & 9 & 26692 & 0.6 & 348.33 & 922.66 & 0.36 & 549.75 & 0.7 & 488.32 & 43.46 \\ \hline
	sym10\_262 & 12 & 28084 & 1 & 176.35 & 1169.6 & 0.48 & 567.8 & 0.8 & 609.1 & 47.82 \\ \hline
	hwb8\_113 & 9 & 30372 & 0.7 & 177.9 & 705.86 & 0.51 & 678.66 & 0.7 & 510.53 & 40.03 \\ \hline
	urf2\_152 & 8 & 35210 & 0.7 & 264.01 & 445.69 & 0.44 & 1056.3 & 0.8 & 558.76 & 41.95 \\ \hline
	 &  & \  & \  & \  & \  & \  & \  & \  & \  & \  \\
	sum &	-	& 333811	& 73.90
	&3821	&13224	&5.21	&4824	&38.90	&6616	&3831\\
    max &	16	& 35210	& 15.40    &503.45	&1516	&0.51	&1056	&5.20	&609	&47.82
    \\ \hline\\
%\end{tabular}
\caption{Comparison on $\mathcal{B}_c$: Time consumption, where `\#q' denotes the number of qubits, '\#CX' the number of \cnot, 'mapp.' and '19mapp.' the topgraph initial mapping construction times on Q Tokyo and Q19x19, respectively, `G' and `GQ01x'  the search time of \fidls-$G$ on Q Tokyo with Q-filter Q01 and Q01x (cf. the last paragraph of Sec.~\ref{sec:eval} on page~\pageref{page:Q01x}), respectively, and `D' the search time of \fidls-$D$ on Q19x19 using Q-filter Q01.  }
\label{tab:b131-time}
\end{longtable}
}
